# Supplementary material for: Low-Complexity Detection of M-ary PSK Faster-than-Nyquist Signaling
Source: arXiv:1810.05443 source file (2019-04-13)
Supplement: Supplementary file 1 [file Appendix.tex]

{ 
\section*{Appendix I: Covariance of noise vector $\bm{\eta}$}
The covariance matrix of the noise vector $\bm{\eta}$ can be calculated as
\begin{eqnarray}\label{eq:main0}
\mathbb{E}\{\bm{\eta}  \bm{\eta}^{\textup{T}}\} &=& \mathbb{E}\{\bm{G}^{-1} \: \bm{q}_{\textup{c}}  \bm{q}_{\textup{c}}^{\textup{T}} \: ({\bm{G}^{-1}})^{\textup{T}}\} \nonumber \\
&=& \bm{G}^{-1} \: \mathbb{E}\{ \bm{q}_{\textup{c}} \bm{q}_{\textup{c}}^{\textup{T}} \} \: ({\bm{G}^{-1}})^{\textup{T}}.
%&=& \bm{G}^{-1} \: \Big(\frac{1}{2} \: \sigma^2 \bm{G}\Big) \: ({\bm{G}^{-1}})^{\textup{T}} \nonumber \\
%&=& \frac{1}{2} \: \sigma^2 \bm{G}^{-1},
\end{eqnarray}
%where $\mathbb{E}\{ \bm{q}_{\textup{c}} \: \bm{q}_{\textup{c}}^{\textup{T}} \} = \frac{1}{2} \: \sigma^2 \bm{G}$ is reached by using $\mathbb{E}\{\Re\{\bm{\overline{q}}\} \Re\{\bm{\overline{q}}\}^{\textup{T}}\} = \mathbb{E}\{\Im\{\bm{\overline{q}}\} \Im\{\bm{\overline{q}}\}^{\textup{T}}\} = \frac{1}{2} \sigma^2 \overline{\bm{G}}$, $\Re\{\overline{\bm{G}}\} = \overline{\bm{G}}$ and $\Im\{\overline{\bm{G}}\} = 0$, and real and imaginary parts of the noise are proper random variables  with equal variance.
Given that the  real noise vector is $\bm{q}_{\textup{c}} = [\Re\{\bm{\overline{q}}\}^{\textup{T}}, \Im\{\bm{\overline{q}}\}^{\textup{T}}]^{\textup{T}}$, the value of $\mathbb{E}\{\bm{q}_{\textup{c}} \bm{q}_{\textup{c}}^{\textup{T}}\}$ can be calculated  as
\begin{eqnarray} \label{eq:main1}
\mathbb{E}\{\bm{q}_{\textup{c}} \bm{q}_{\textup{c}}^{\textup{T}}\} & = &  \begin{bmatrix}
\mathbb{E}\{\Re\{\bm{\overline{q}}_{\textup{c}}\} \Re\{\bm{\overline{q}}_{\textup{c}}\}^{\textup{T}}\} & \mathbb{E}\{\Re\{\bm{\overline{q}}_{\textup{c}}\} \Im\{\bm{\overline{q}}_{\textup{c}}\}^{\textup{T}}\}\\
\mathbb{E}\{\Im\{\bm{\overline{q}}_{\textup{c}}\} \Re\{\bm{\overline{q}}_{\textup{c}}\}^{\textup{T}}\} & \mathbb{E}\{\Im\{\bm{\overline{q}}_{\textup{c}}\} \Im\{\bm{\overline{q}}_{\textup{c}}\}^{\textup{T}}\}
\end{bmatrix}. \nonumber \\
\end{eqnarray}
The values of $\mathbb{E}\{\Re\{\bm{\overline{q}}_{\textup{c}}\} \Re\{\bm{\overline{q}}_{\textup{c}}\}^{\textup{T}}\} $ and $\mathbb{E}\{\Re\{\bm{\overline{q}}_{\textup{c}}\} \Im\{\bm{\overline{q}}_{\textup{c}}\}^{\textup{T}}\}$
%, $\mathbb{E}\{\Im\{\bm{\overline{q}}_{\textup{c}}\} \Re\{\bm{\overline{q}}_{\textup{c}}\}^{\textup{T}}\}$, and $\mathbb{E}\{\Im\{\bm{\overline{q}}_{\textup{c}}\} \Im\{\bm{\overline{q}}_{\textup{c}}\}^{\textup{T}}\}$ 
can be calculated with the help of $ \mathbb{E}\{\bm{\overline{q}}_{\textup{c}} \bm{\overline{q}}_{\textup{c}}^{\textup{H}}\} = \sigma^2 \overline{\bm{G}}$ as follows.
\begin{eqnarray}
 \mathbb{E}\{\bm{\overline{q}}_{\textup{c}} \bm{\overline{q}}_{\textup{c}}^{\textup{H}}\} &=&  \mathbb{E}\{(\Re\{\bm{\overline{q}}_{\textup{c}}\} + j \Im\{\bm{\overline{q}}_{\textup{c}}\}) (\Re\{\bm{\overline{q}}_{\textup{c}}\}^{\textup{T}} - j \Im\{\bm{\overline{q}}_{\textup{c}}\}^{\textup{T}})\} \nonumber \\
&=&  \mathbb{E}\{\Re\{\bm{\overline{q}}_{\textup{c}}\} \Re\{\bm{\overline{q}}_{\textup{c}}\}^{\textup{T}}\} + \mathbb{E}\{\Im\{\bm{\overline{q}}_{\textup{c}}\} \Im\{\bm{\overline{q}}_{\textup{c}}\}^{\textup{T}}\} \nonumber \\ & &  + j \mathbb{E}\{\Im\{\bm{\overline{q}}_{\textup{c}}\} \Re\{\bm{\overline{q}}_{\textup{c}}\}^{\textup{T}}\} - j \mathbb{E}\{\Re\{\bm{\overline{q}}_{\textup{c}}\} \Im\{\bm{\overline{q}}_{\textup{c}}\}^{\textup{T}}\}. \nonumber \\ 
& = & \sigma^2 \overline{\bm{G}} \label{eq:3}
\end{eqnarray}
We assume that $\mathbb{E}\{\Im\{\bm{\overline{q}_{\textup{c}}}\} \Re\{\bm{\overline{q}_{\textup{c}}}\}^{\textup{T}}\} = \mathbb{E}\{\Re\{\bm{\overline{q}_{\textup{c}}}\} \Im\{\bm{\overline{q}_{\textup{c}}}\}^{\textup{T}}\} = 0$ (this assumption can be further verified from the fact that $p(t)$ is real-valued, and hence, $\Im\{\overline{\bm{G}}\} = 0$ for the considered AWGN case; accordingly, $\sigma^2 \overline{\bm{G}}$ does not have imaginary parts). Accordingly, \eqref{eq:3} is re-written as
%For the transmission scenario discussed in this paper, we have $\Im\{\overline{\bm{G}}\} = 0$. Hence, we can write
\begin{eqnarray}
\mathbb{E}\{\Re\{\bm{\overline{q}}_{\textup{c}}\} \Re\{\bm{\overline{q}}_{\textup{c}}\}^{\textup{T}}\} + \mathbb{E}\{\Im\{\bm{\overline{q}}_{\textup{c}}\} \Im\{\bm{\overline{q}}_{\textup{c}}\}^{\textup{T}}\}  &=&  \sigma^2 \overline{\bm{G}}.
\end{eqnarray}
We also assume that the noise is a proper random variable, i.e. its real and imaginary parts  have equal variance \cite{neeser1993proper}; that said we can conclude  that
\begin{eqnarray}
\mathbb{E}\{\Re\{\bm{\overline{q}}_{\textup{c}}\} \Re\{\bm{\overline{q}}_{\textup{c}}\}^{\textup{T}}\} = \mathbb{E}\{\Im\{\bm{\overline{q}}_{\textup{c}}\} \Im\{\bm{\overline{q}}_{\textup{c}}\}^{\textup{T}}\}   =  \frac{1}{2} \sigma^2 \overline{\bm{G}}. \label{eq:5}
\end{eqnarray}
By substituting \eqref{eq:5} into \eqref{eq:main1}, we get
\begin{eqnarray} \label{eq:main2}
\mathbb{E}\{\bm{q}_{\textup{c}} \bm{q}_{\textup{c}}^{\textup{T}}\} & = &  \begin{bmatrix}
\frac{1}{2} \sigma^2 \overline{\bm{G}} & 0\\
0 & \frac{1}{2} \sigma^2 \overline{\bm{G}}
\end{bmatrix}, \nonumber \\
& = & \frac{1}{2} \sigma^2 {\bm{G}},
\end{eqnarray}
which is reached by  knowing that $\Re\{\overline{\bm{G}}\} = \overline{\bm{G}}$ and $\Im\{\overline{\bm{G}}\} = 0$ for the considered AWGN case. Finally, from \eqref{eq:main0} and \eqref{eq:main2}, one can easily find that $\mathbb{E}\{\bm{\eta}  \bm{\eta}^{\textup{T}}\}  =  \frac{1}{2} \: \sigma^2 \bm{G}^{-1}$.
}
